# Supplementary material for: Action-slot: Visual Action-centric Representations for Multi-label Atomic Activity Recognition in Traffic Scenes
Source: arXiv:2311.17948 source file (2024-04-20)
Supplement: Supplementary file 1 [file X_suppl.tex]

\clearpage
\setcounter{page}{1}
%\maketitlesupplementary
